# Supplementary material for: Reinforcement Learning for Mean Field Game
Source: arXiv:1905.13357 source file (2019-10-08)
Supplement: Supplementary file 1 [file appendix.tex]

\appendixpage
\appendix
\setcounter{page}{1}

\section{Dynamic Programming Equations for Finite-Horizon MDPs }\label{dyn_mdp}

We define the value function at $l^{th}$ time step as:
\begin{align}
    V_{\pi,\ell}(s|\alpha) &= \mathbf{E}_{{\cal M},\pi}\left[\sum_{j=\ell}^{\tau-1}\gamma^{j-\ell}\Bar{r}(s_{j}, \pi(s_{j},j), \alpha)|s_\ell = s, \pi\right]
\end{align}
This can be further re-written as 
\begin{align}
    V_{\pi,\ell}(s|\alpha)&= \mathbf{E}_{{\cal M},\pi}\left[\Bar{r}(s, \pi(s,\ell), \alpha) + \sum_{j=\ell+1}^{\tau-1}\gamma^{j-\ell}\Bar{r}(s_{j}, \pi(s_{j},j), \alpha)|s_{\ell+1} = s, \pi\right]
\end{align}
Separating the two terms inside the expectation and taking $\gamma$ outside the expectation, we get
\begin{align}
    V_{\pi,\ell}(s|\alpha) &= \mathbf{E}_{{\cal M},\pi}\left[\Bar{r}(s, \pi(s,\ell), \alpha)\right] + \gamma\mathbf{E}_{{\cal M},\pi}\left[\sum_{j=\ell+1}^{\tau-1}\gamma^{j-(\ell+1)}\Bar{r}(s_{j}, \pi(s_{j},j), \alpha)|s_{\ell+1} = s, \pi\right]
\end{align}

After choosing the action $\pi(s,\ell)$ in state $s$, the agent transitions to the state $s'$ with transition probability $p(s'|s,\pi(s,\ell),\alpha)$.
\begin{align}
    V_{\pi,\ell}(s|\alpha) &= \Bar{r}(s, \pi(s,\ell), \alpha) + \gamma\sum_{s'\in S}p(s'|s,\pi(s,\ell+1),\alpha)\mathbf{E}_{{\cal M},\pi}\left[\sum_{j=\ell+1}^{\tau-1}\gamma^{j-(\ell+1)}\Bar{r}(s_{j}, \pi(s_{j},j), \alpha)|s_{\ell+1} = s', \pi\right]
\end{align}
But $V_{\pi,\ell+1}(s'|\alpha) = \mathbf{E}_{{\cal M},\pi}\left[\sum_{j=\ell+1}^{\tau-1}\gamma^{j-(\ell+1)}\Bar{r}(s_{j}, \pi(s_{j},j), \alpha)|s_{\ell+1} = s', \pi\right]$, which gives 
\begin{align}
    V_{\pi,\ell}(s|\alpha= \Bar{r}(s, \pi(s,\ell), \alpha) + \gamma\sum_{s'\in S}p(s'|s,\pi(s,\ell+1),\alpha)V_{\pi,\ell+1}(s'|\alpha)
\end{align}
Thus, the above defined value functions  satisfy the dynamic programming equations for finite-horizon MDPs.

\if 0
\section{Thompson Sampling Lemma}

\begin{lem}($\cite{osband}$)
Suppose $H_{t_k}$ denotes the history till time $t_k$. Any $\sigma-$ measurable function of $H_{t_k}$, $g$ satisfies the following
\begin{align}\label{eq:truevsmdp}
\mathbf{E}[g({\cal M}_k)|H_{t_k}]=\mathbf{E}[g({\cal M}^*)|H_{t_k}]
\end{align}
where ${\cal M}^*$ is the true transition probability.  \label{lem:expec}
\end{lem}

Conditioned on $H_{t_k}$, the only randomness in the function $g(\mathcal{M_k})$ comes form the random sampling in the Algorithm 1. This gives us the following equation:
\begin{eqnarray}
&& \mathbf{E}[g({\cal M}_k))] \\
&=& \mathbf{E}[g({\cal M}_k)) | H_{t_k}, \pi_k, t_k]\\
 &=& \int g({\cal M}_k)) | H_{t_k}, \pi_k, t_k]\pi_k(d\mathcal{M})\\
 &=& \mathbf{E}[g({\cal M}^*)|H_{t_k}]
\end{eqnarray}
The last step comes from the fact that $\pi_k$ is the posterior distribution of $\mathcal{M}^*$ given $H_{t_k}$.

Note that by the tower property, 
\begin{align}\label{eq:sm}
    \mathbf{E}[g({\cal M}_{t_k})]=\mathbf{E}[g({\cal M}^*)]
\end{align}
Here ${\cal M}_{t_k}$ is any sampled distribution of an agent at time $t_k$.

\section{Proof of Lemma \ref{value_increase}}\label{apdx_value}
%We note that at each time only one agent changes the policy. For a given strategy of all other users, the change of the strategy of the agent only happens to update the value function. We note that even when the actions were not taken, the value function was kept updating giving it a better estimate of the true value function. As seen later in the proof of Theo, we show that the updates of the value function give an accurate estimate of the value function. Thus, when the policy is modified to the one optimizing the estimated value function, the policy improves the overall value function. 
Since the change happens for one agent at a time, and the fact that a single agent does not impact the $\alpha$ of other users, the rewards of the other users are not impacted and thus remain the same. Since the agent that modified the policy must have increased value function by changing the policy (cannot be the same due to the choice of the infimum of $\mathcal{P}(\alpha_{t_k})$), the reward will only increase if the policy is modified. Thus, the overall value function by the update of a single agent is non-decreasing. 

% not impacting their reward significantly while increasing the expected reward of the user which changed the policy. Thus, the overall value function is non-decreasing. 
%\fi 
\section{Azuma-Hoeffding}\label{apx:azuma}

\begin{lem}(Azuma-Hoeffding Lemma \cite{osband}) If $ Y_{n} $ is a zero-mean martingale with almost surely bounded increments, $|Y_{i}$ -  $Y_{i-1}|$ $\leq$ C, then for any $\delta$ $\geq$ 0 with probability at least 1-  $\delta$, $Y_{n} \leq C\sqrt{2n\log(1/\delta)}$. \label{lem:azuma}
\end{lem}

%\if 0
\section{Expected SARSA: Conditions on $F_t$}

\begin{lem}\label{sarsa}
Consider a stochastic process ($\Delta_n(x)$, $\zeta_n(x)$, $F_n(x)$), etc. Need citation for the result. A random iterative process $\Delta_{n+1}(x)$ = $(1 - \zeta_n(x))\Delta_n + \zeta_n(x)F_n(x)$ converges to zero under the following assumptions: 
\begin{enumerate}
    \item The state space is finite
    \item $\sum_{n}\zeta_n(x) = \infty$, $\sum_{n}^{2}\zeta_n(x) < \infty$
    \item $|| E[\{F_n|P_n\}] ||_W  \leq \kappa||\Delta_n||_W + c_n, $ where $ \kappa \in (0,1)$ and $c_n$ converges to zero.
    \item Var$\{F_n|P_n\} \leq C(1 + \kappa||\Delta_n||^{2}_{W})$, where C is some constant.
\end{enumerate}

Here $P_n$ is a sequence of increasing $\sigma$ -fields  such  that $\zeta_0$ and $\Delta_0$ are $P_0$-measurable and $\zeta_n$, $\Delta_n$ and $F_n$ are $P_n$-measurable, $n \geq 1.$  \label{lem:zeta}
\end{lem}

%The above lemma is used often to show the of convergence of stochastic iterative dynamic programming algorithms and can be similarly used here to show the convergence of the $Q$ functions to the optimal value.
%We, now, introduce a notation which we use throughout this section. 
We have defined the random stochastic process $\epsilon^j_{k}(s_t,a_t,\alpha)$ given by:
\begin{align}
\epsilon^j_{k+1}(s_t,a_t,\alpha)=(1-\beta_k)\epsilon^j_{k}(s_t,a_t,\alpha)+\beta_k F_k(s_t,a_t,\alpha), 
\end{align}
where, $F_k(s_t,a_t,\alpha) = r^j_k(s_t,a_t,\alpha)+\gamma v^j_k(s_{t+1}|\alpha)$.
It is obvious that time $t = (k-1)\tau +j$.
We will now show that $\max_s\max_a|\epsilon^j_k| \rightarrow 0$ as $t \rightarrow 0.$  We will now show that $||\mathbf{E}[F^j_k]|| \leq \kappa||\epsilon^j_k|| + c_k$ where $\kappa \in [0,1]$ and $c_t$ converges to zero which will fulfill the conditions 3 and 4 of Lemma \ref{sarsa}. % and we can show that $\epsilon_t$ converges to zero.\\
We proceed as follows:
\begin{eqnarray} 
&&||\mathbf{E}[F^j_k]|| \nonumber\\
 & \stackrel{(a)}{=}& ||\mathbf{E}[r^j_k + \gamma\sum_a\pi_k(s_{t+1}, a)q^j_k(s_{t+1},a,\alpha) - Q^{\mathcal{M}_k}_{\pi_k,j}(s_t,a_t,\alpha)]||\\
 & \stackrel{(b)}{=}& ||\mathbf{E}[r^j_k + \gamma\sum_a\pi_k(s_{t+1}, a)q^j_k(s_{t+1},a,\alpha) + \gamma \max_aq^j_k(s_{t+1},a,\alpha) - \gamma \max_aq^j_k(s_{t+1},a,\alpha) \nonumber\\
 && - Q^{\mathcal{M}_k}_{\pi_k,j}(s_t,a_t,\alpha)]||\\
 &\stackrel{(c)}{\leq}& ||\mathbf{E}[r^j_k + \gamma \max_aq^j_k(s_{t+1},a,\alpha) - Q^{\mathcal{M}_k}_{\pi_k,j}(s_t,a_t,\alpha)]|| \nonumber \\
 &&+   \gamma\mathbf{E}\left[\sum_a\pi_k(s_{t+1}, a)q^j_k(s_{t+1},a,\alpha) - \max_aq^j_k(s_{t+1},a,\alpha)\right] \\
 & \stackrel{(d)}{\leq}& \gamma \max_s\left|\max_a q^j_k(s,a) - \max_a Q^{\mathcal{M}_k}_{\pi_k,j}\right| \nonumber  \\
 &&+ \gamma \max_s\left|\sum_a\pi_k(s,a)Q_t(s,a) - \max_aq^j_k(s,a)\right|\\
 & \stackrel{(e)}{\leq}& \gamma||\epsilon_k|| + \gamma \max_s\left|\sum_a\pi_k(s,a)q^j_k(s,a) - \max_aq^j_k(s,a)\right|\\
 & =& \kappa||\epsilon_k|| + c^j_k,
\end{eqnarray}

Here, (a) follows from Eq. (25), (b) follows by subtracting and adding the term $\gamma \max_aq^j_k(s_{t+1},a,\alpha)$ inside the expected value, (c) follows by applying the inequality $||a+b|| \leq ||a|| + ||b|| $ and separating the two terms inside the expected value.

Now we use the definition of $Q^{\mathcal{M}_k}_{\pi_k,j}(s_t,a_t,\alpha)$ which is defined as\\ $Q^{\mathcal{M}_k}_{\pi_k,j}(s_t,a_t,\alpha) = r^j_k + \gamma \max_aQ^{\mathcal{M}_k}_{\pi_k,j}(s_{t+1},a,\alpha)$.

We also use the fact that difference of the two value at state $s_{t+1}$ is less than the maximum possible value, which is gives us (d) and (e) follows by substituting the value of $\epsilon^j_k$ from Eq. (21).

We have $c^j_k$ = $\gamma \max_s |\sum_a \pi_t(s,a)Q_t(s,a) -\max_aQ_t(s,a)|$ and $\kappa = \gamma$. Clearly for all policies that are greedy in limit {\bf Unclear}, $c_t$ converges to zero. Therefore, for $\gamma < 1$, all conditions of Lemma \ref{sarsa} follow and we can apply the lemma to prove the convergence of $Q_t$ to $Q^*$.
\fi
